# Supplementary material for: Unraveling Modular Microswimmers: From Self-Assembly to Ion-Exchange Driven Motors
Source: arXiv:1807.10175 source file (2018-12-03)
Supplement: Supplementary file 1 [file Supplementary_information.pdf]

Supplementary Information

# Unraveling Modular Microswimmers: From Self-Assembly to Ion-Exchange Driven Engines

Benno Liebchen[1,*], Ran Niu[2,*], Thomas Palberg[2] and Hartmut Löwen[1]

1. Institut für Theoretische Physik II: Weiche Materie, Heinrich-Heine-Universität Düsseldorf, D-40225 Düsseldorf, Germany

2. Institut für Physik, Johannes Gutenberg-Universität Mainz, Staudingerweg 7, D-55128 Mainz, Germany

## 1. Methods

### 1.1 Electrokinetic equations

To understand the motion of a colloidal particle in the fields produced by the ion-exchange resin (ionic density, solvent velocity and electrostatic potential), we consider a standard set of electrokinetic equations in 3D, which we then simplify and partly solve in 2D and confined 3D geometries below. The time-evolution of the density field of ions $c_i$ of species $i \in (H^+, K^+, Cl^-)$ (see setup) and diffusion coefficient $D_i$ follows the Nernst-Planck equation:

$$\dot{c}_i = -\nabla \cdot \mathbf{j}_i; \quad \mathbf{j}_i = -D_i \nabla c_i + \mathbf{u} c_i - \frac{eZ_i}{kT} D_i c_i \nabla \psi \qquad (8)$$

where $\psi$ is the electrostatic potential and $\mathbf{u}$ is the velocity field of the underlying solvent. This equation has the form of a conservation equation expressing the fact that the ionic density fields are conserved (in bulk).

The Poisson equation describes the electrostatic potential produced by a given distribution of ions

$$-\varepsilon \nabla^2 \psi = \sum_i Z_i e c_i \qquad (9)$$

and the Stokes equation determines the solvent flow as produced by the stress generated by the action of the electric field on the charged fluid in the interfacial layer of the substrate

$$\eta \nabla^2 \mathbf{u} - \nabla p = -\sum_i e Z_i c_i \nabla \psi \qquad (10)$$

which has to be solved simultaneously with the solvent incompressibility condition

$$\nabla \cdot \mathbf{u} = \mathbf{0} \qquad (11)$$

Equations (8–11) constitute a complete set of equations determining, together with appropriate boundary conditions, all field, $c_{H^+}$, $c_{K^+}$ $c_{Cl^-}$, $p$, $\mathbf{u}$, $\psi$. While a complete solution of these equations is challenging, even numerically [1], here we focus on the derivation of approximate analytical expressions to the extend needed to broadly understand the self-assembly, exclusion zone formation and swimming speed of modular swimmers.

### 1.2 Spontaneous electric field: Impact of solvent flow

Here we derive the electrostatic potential for given ionic concentration gradients which we then determine in

later sections. To avoid a co-current diffusion of co- and counterions, we must require $\mathbf{j}^{+}=\mathbf{j}^{-}$, where $\mathbf{j}^{\pm}$ denotes the sum of the ionic currents of all positive/negative species. Combining this condition with Eq. (8), we find

$$\nabla\psi=\frac{\sum_{-} D_i\nabla c_i-\sum_{+} D_i\nabla c_i+\mathbf{u}\left[\sum_{+} c_i-\sum_{-} c_i\right]}{\sum_{+} Q_i D_i c_i-\sum_{-} Q_i D_i c_i} \qquad (12)$$

where $\sum_{+,-}$ represent sums over all positively and negatively charged species respectively and $Q_i = eZ_i/(kT)$.

Thus, an *electric field emerges spontaneously* arising as a consequence of the exchange of ions with different mobilities by the resin. This unscreened electric field is the key player here whereas the direct electric field created by the charges (colloids, resin, substrate) decays on a length scale of the Debye screening length. The Debye length is short compared to the colloid radius and the plate thickness, even for the low ionic concentrations in the present experiment (If direct electrostatic interactions were important here, they should lead to a significant equilibrium distance between the colloids, which is not observed experimentally). Thus, on relevant length scales, Eq. (9) essentially reduces to $\sum_i Z_i e c_i \approx 0$, i.e. since $|Z_i = 1|$ for all *i*, we have $\sum_{+} c_i = \sum_{-} c_i$ outside the Debye layer. Thus, the term in square brackets in Eq. (12) vanishes, showing, remarkably, that solvent advection has no influence on the relation between the spontaneously emerging electric field and the ionic distributions. Physically, this is because solvent advection transports all ions in the same direction and therefore does not contribute to charge imbalances, unless for ions of unequal charge magnitude.

For the present case of three single-charged ionic species, we have $Z_i^2$ =1 for all species and outside the Debye layer also $c_{Cl^-} = c_{H^+} + c_{K^+}$. Thus, Eq. (12) simplifies to:

$$\nabla\psi=\frac{kT}{e}\frac{(D_{Cl^-}-D_{H^+})\nabla c_{H^+}+(D_{Cl^-}-D_{K^+})\nabla c_{K^+}}{(D_{Cl^-}+D_{H^+})c_{H^+}+(D_{Cl^-}+D_{K^+})c_{K^+}} \qquad (13)$$

For the present case, where we have $D_{K^+} \approx D_{Cl^-}$ and $c_{K^+} \gg c_{H^+}$ (far away from the resin, we have $c_{K^+} \approx 1$ µmol/L and $c_{H^+} \approx 0.1$ µmol/L [1]), we can write

$$\nabla\psi \approx \frac{-kT}{e}\mathrm{D}\frac{\nabla c_{H^+}}{c_{K^+}} \qquad (14)$$

where $\mathrm{D} = \left(D_{H^+}-D_{K^+}\right)/\left(2D_{K^+}\right)$.

## 1.3 Solvent Flow

Having shown that solvent advection of the ions does not influence the relation between ionic-concentration profiles and the spontaneously emerging electric field $\mathbf{E}=-\nabla\psi$, but only the ionic fields themselves, we can now essentially follow standard theories [2] to derive the solvent velocity as caused by a given, externally controlled, concentration gradients. We first perform a local near-equilibrium approximation assuming that the ion-distribution of each species perpendicular to the glass plate follows a Boltzmann-distribution $c_i(\rho,z)=c_i^{\infty}(\rho)\exp\left\{\left[\frac{-Z_i e}{kT}\left(\psi(\rho,z)-\psi^{\infty}(\rho)\right)\right]\right\}$, where *z* is the distance to the (lower) glass plate and ρ is the distance from the resin surface along the glass plate. The ∞-superscript represents evaluation of concerned fields at *z*-values outside the double layer of the substrate and is omitted in the following (The specific *z*-value

does not matter in this regime if $\rho \gg z$). Thus, the ionic density of the positive counterion cloud to the negatively charged glass substrate is maximal close to the substrate and then decays exponentially on the scale of a Debye length. The fluid elements inside the double layer of the lower glass substrate are charged and experience a stress due to the spontaneously emerging electric field leading to a fluid flow. We can approximately calculate this flow from the Stokes equation

$$-\eta\nabla^2\mathbf{v} + \nabla p + (c_{H^+} + c_{K^+} - c_{Cl^-})e\nabla\psi = 0 \quad (15)$$

Following [2], we first integrate the Stokes equation in $z$-direction, leading to

$$p(\rho,z) = 2kTc_{Cl^-}(\rho)\left\{\cosh\left[\frac{e}{kT}(\psi(\rho,z) - \psi^\infty(r))\right] - 1\right\}\partial_\rho c_{Cl^-}(\rho)$$

(Note that we have $c_{Cl^-} \approx c_{H^+} + c_{K^+}$). Now combining this expression for the pressure with the standard Poisson-Boltzmann equation $\tanh(\phi(\rho,z)/4) = \gamma exp[-\kappa(\rho)z]$ with $\gamma = \tanh(e\zeta/(4kT))$ and the (local) inverse Debye length $\kappa(\rho) = \left[8\pi e^2 c_{Cl^-}(\rho)/(\varepsilon kT)\right]^{1/2}$, plugging the result into the Stokes equation, integrating twice (compare [2]), and using (14) leads to the following slip velocity relative to the glass substrate:

$$\mathbf{v}_a(\rho) = \frac{-\varepsilon kT}{4\pi\eta e}\left[\zeta \mathrm{D}\frac{\partial_\rho c_{H^+}}{c_{K^+}} - 2\frac{kT}{e}\ln(1-\gamma^2)\frac{\partial_\rho c_{Cl^-}}{c_{Cl^-}}\right]\mathbf{e}_\rho \quad (16)$$

where $\mathbf{e}_\rho$ is the unit vector pointing radially away from the resin surface in the plane of the glass plate. The first part in Eq. (16) is similar to the corresponding result for the slip velocity in [1] but not identical; the second term, which is equally important here according to our parameter estimates below, is neglected in [1]. Note that the same expression holds true for the slip velocity on the colloidal surface, but with the ζ-potential of the glass plate being replaced with that of the colloid. Note that $\kappa R_c \gg 1$ as can be seen directly by pH measurements and also indirectly since the colloids stay at close contact to each other suggesting that direct electrostatic interactions are unimportant.

In the next paragraph we will discuss the shape of the chemical fields and gradients. In the experiment we have a background ion density, far away from the resin, of $c^0_{K^+} \approx$ 1.0 μmol/L and $c^0_{H^+} \approx$ 0.1 μmol/L and $c^0_{Cl^-} \approx c^0_{H^+} + c^0_{K^+}$, so that $\frac{\partial_\rho c_{H^+}}{c_{K^+}} \approx \frac{\partial_\rho c_{H^+}}{c^0_{K^+}}$ and $\frac{\partial_\rho c_{Cl^-}}{c_{Cl^-}} \approx \frac{\partial_\rho c_{Cl^-}}{c^0_{Cl^-}}$.

## 1.4 Slip velocity: Far-field scaling of the chemical gradients

Here we approximately calculate the chemical fields both at large and short distances to the resin, to understand the far-field scaling and the saturation value of the solvent advection velocity. While in general, the density profiles of the ions are influenced by both the spontaneous electrostatic field and the subsequent solvent advection (Eq. 8), here we use a much-simplified framework. Physically, this approach may be motivated by the fact that the exchange and diffusion of ions with different mobilities should dominate over its consequences (emergence of a spontaneous electric field and solvent flow) and should therefore produce the dominant contribution in Eq. (8); otherwise the fields would self-amplify or self-destroy in a feedback loop. More formally, Eq. (12) show that the electrostatic term in the Nernst-Planck equation (Eq. 8), can be approximately absorbed in the diffusion term, leading to (slightly[1]) a renormalized diffusion coefficient, not affecting scaling laws. The impact of solvent advection on the concentration fields in turn is discussed more explicitly below and can be neglected for our purposes.

Here, we first explore the far field regime, where we can describe the resin essentially as a point source (at

---

[1] Far away from the resin, the correction to the diffusion coefficient is of order $c_{H^+}/c_{K^+} + \mathrm{D} \ll 1$; closer to the resin it might have a relevant quantitative impact.

the origin) exchanging $K^{+}$-ions with $H^{+}$-ions with a rate $kc_{K^{+}}(\mathbf{r}=\mathbf{0}) \approx kc^{0}_{K^{+}} =: k_0$. In free 3D space, we calculate the distribution of $H^{+}$-ions from the following diffusion equation ( $D := D_{H^{+}}$ being the diffusion constant of $H^{+}$-ions in water):

$$\dot{c} = D\nabla^2 c + k_0\delta(\mathbf{r}) \quad (17),$$

whose steady state solution is $c(r) = k_0/(4\pi D r)$ [3].

In the present experiment, besides the backaction of the spontaneous electric field onto the ionic gradients, there are two relevant changes to this scenario, namely fluid advection and confinement. Remarkably, fluid advection is unlikely to change the ion-distribution significantly. This can be seen, when considering Eq. (17) with an additional (constant) advection term $-\mathbf{u}_0 \cdot \nabla c$ on the right hand side of Eq. (17), leading to [3]: $c(\mathbf{r}) = \left[k_0/(4\pi D r)\right]\exp\left[-\left(|\mathbf{u}_0 r| - \mathbf{u}_0 \cdot \mathbf{r}\right)/(2D)\right]$. For typical parameters $D\sim 10^4$ µm²/s; $|\mathbf{u}|_0 \lesssim 5$ µm/s and at colloid-resin-distances $r \lesssim 100$ µm *as* for the self-assembly process, we have $|\mathbf{u}|_0\, r/(2D) \lesssim 0.03$, so that the quantitative impact of advection on the shape of the ionic gradients is probably not relevant at length scales relevant for the swimmer self-assembly here. (Note that this finding somewhat contrasts with [1] where a Peclet number Pe= $|\mathbf{u}|_0\, L/D>1$, with $L\sim 1\text{-}10$ mm being the cell height, has been introduced to suggest that neglecting solvent advection may be inappropriate to understand the ionic gradients even at distances <100 µm to the resin. The present consideration suggests, however, that the impact of solvent advection on the ionic concentration gradients is very minor at such length scales. Only at very large distances to the resin (order of magnitude 1 mm) solvent advection should be important since $|\mathbf{u}|_0\, r/(2D)\sim 1$. In addition to this, applying scaling arguments to the above electrokinetic equations suggests that advection helps localizing the concentration profiles around the resin at mm scales; in bulk 3D for example, we find that advection should change the $1/r$-shape towards $1/r^2$ shapes; physically, this is probably because advection effectively pushes the ionic fields towards the resin.

In contrast to advection, confinement has a significant impact on the shape of the ionic-fields even at distances relevant for the self-assembly process of modular swimmers. The present experiment takes place between two parallel glass plates at a distance $L$. Considering a point source at a distance of $R_{\mathrm{IEX}}$ above the lower glass plate (at $z$=0), the steady-state solution of the confined 3D-diffusion problem does diverge (see also [1]). To reach a steady state, the ionic exchange (production) rate must either slow down (this happens in our experiments on the timescale of days) or decay ("evaporate") due to boundary absorption processes/secondary reactions due to imperfect purity or other loss processes. Both cases essentially lead to a $1/\rho$-far field scaling law as we show in the following:

**Case 1: Decay-processes** Here, we add a (pseudo-)decay term $-k_d c$ to the diffusion equation, allowing the system reaching a steady state. The corresponding steady state solution reads:

$$c(r) = \frac{k_0}{4\pi D}\left[\sum_{n=0}^{\infty}\frac{\exp\left[-\tilde{\kappa}\sqrt{\rho^2+(z+R+2nL)^2}\right]}{\sqrt{\rho^2+(z+R+2nL)^2}} + \sum_{n=0}^{\infty}\frac{\exp\left[-\tilde{\kappa}\sqrt{\rho^2+(z-R+2nL)^2}\right]}{\sqrt{\rho^2+(z-R+2nL)^2}}\right] \quad (18)$$

While we cannot solve the corresponding sums, for distances $\rho>L/2$, numerical evaluation of the two sums shows that their sum can be closely approximated by $2K_0(\tilde{\kappa}\rho)/L$ where $\rho$ is the distance to the source along (parallel to) the lower plate, $\tilde{\kappa} = \sqrt{\kappa_d / D}$ is an effective inverse screening length and $K_0$ is the 0-th modified

Bessel function of the second kind (MacDonald function). (Even for distances $\rho$ significantly smaller than $L/2$ the present approximation is useful – but not for distances $\rho \ll L$). For very small decay-rates (so that $\sqrt{k_d / D}\rho \ll 1$ )

we have $K_0(\tilde{\kappa}\rho) = const - \ln(\tilde{\kappa}\rho)$. Thus, far away from the resin, when $\tilde{\kappa} \ll 1$ (i.e. when the ionic-decay rate is very small) we obtain:

$$\partial c_{H^+} / c_{K^+} \approx \frac{K_0(\tilde{\kappa}\rho)}{2\pi D_c L c^0_{K^+} \rho} \qquad (19)$$

leading to a $1/\rho$-speed for the advection speed far away from the resin. We obtain the same result when using the 2D diffusion equation with a decay-term, corresponding to the fact that the present confined geometry essentially looks like a 2D problem when viewing it from large distances. Accordingly, if the box is too high and $\rho \ll L$ the above expansion is no longer justified and the diffusion problem is essentially 3D; at relevant distances, we then obtain $\partial c_{H^+} / c_{K^+} \propto 1/\rho^2$. In addition, as mentioned above, very far from the resin (order of magnitude 1 mm) solvent advection should change the shape of the gradients favouring a $1/\rho^2$ behaviour.

**Case 2:** In case absorption/decay processes are completely absent, the only process allowing the system to reach steady state chemical concentration gradients is the slow-down of the production. Solving the time-dependent 2D version of Eq. (17) asymptotically at large $t$ and a constant production rate, we obtain

$$c = -k_0 \ln\left[\rho^2/(4Dt)\right]/(4D) \quad (20)$$

Since the time-dependence of the production is much slower than the intrinsic timescale of the diffusion-process we can simply replace $k_0 \to k_0(t)$ in Eq. (20). From Eq. (20), we obtain $\partial_\rho c = -k_0 / (2D\rho)$, showing that a slowdown of the production leads to a $1/\rho$-scaling law analogously to Case 1. Note that following Eq. (20), reaching a steady state in the complete absence of absorption/decay processes, $\kappa_d = 0$, would require an at least logarithmically fast decay of $k_0$.

## 1.5 Near Field Approximation of the Chemical Density

Here we provide a simple model to approximately calculate the ionic gradients close to the resin (observed e.g. in [1]), allowing us to estimate the saturation values of the solvent advection and the phoretic motion of the colloid. Here we describe the resin as an extended spherical source emitting $H^+$-ions with a uniform rate on its surface; we assume the emission rate to be constant on relevant timescales since $c_{K^+} \approx c^0_{K^+}$. (Conversely to the previous section, for the near-field, where $\rho \ll L$, the upper boundary plays essentially no role, so that the system still reaches a steady state.)

The chemical field as produced by a spherical source can be calculated by distributing point-sources on a sphere, yielding

$$c(r) = \frac{k_0 / S}{4\pi D} \int_{|\mathbf{r}'|=R_{IEX}} \frac{1}{|\mathbf{r} - \mathbf{r}'|} d^3 r' \quad (21)$$

where $S = 4\pi R^2_{IEX}$ is the surface of the resin and the integral is performed over all points on its surface. Now choosing a coordinate system whose origin is at the centre of the sphere and whose $z$-axis is parallel to $\mathbf{r}$, i.e. $\mathbf{r}=(0,0,z)$, using spherical coordinates $\mathbf{r}' = r'(\sin\theta\cos\phi, \sin\theta\sin\phi, \cos\theta)$, we find

$$c(r) = \frac{k_0 / S}{4\pi D} \int_0^{2\pi} d\phi \int_0^{\pi} d\theta \int_0^{\infty} dr' \frac{r'^2 \sin\theta \delta(r' - R_{IEX})}{\sqrt{r'^2 + z^2 - 2r'z\cos\theta'}} = \frac{k_0}{2\pi D}\left(\frac{1}{|R_{IEX} + z| + |R_{IEX} - z|}\right) \quad (22)$$

where $z$ is the distance from the resin centre. Since the resin lies on top of a substrate, we need to account for no-flux boundary conditions at the substrate surface. Therefore, we switch back to cylinder coordinates $(\rho, \phi, z)$ where the substrate defines the $z$=0 plane with the resin-centre now being at $\rho$= 0, z= $R_{IEX}$. In these coordinates,

$c(r)$ has the same form as given in Eq. (1) after replacing $z \to |\mathbf{r} - R_{IEX}\mathbf{e}_z|$. To accomplish no-flux boundary conditions, we can now simply add a spherical mirror-source with midpoint at $z= -R_{IEX}$ and obtain, specifically for z= $R_C \ll R_{IEX}$:

$$c(\rho) = \frac{k_0}{\pi D} \frac{1}{\sqrt{\left(\sqrt{\rho^2 + R_{IEX}^2} + R_{IEX}\right)^2} + \sqrt{\left(\sqrt{\rho^2 + R_{IEX}^2} - R_{IEX}\right)^2}} \quad (23)$$

Note that we have neglected the presence of the upper glass-plate, which plays only a very minor role for the near field behavior of $c(\rho)$, since $\sqrt{\rho^2+z^2} \ll L$. To calculate the saturation value of the fluid advection speed close to the resin surface, we specifically need the maximum of $\partial_\rho c(\rho)$. Specifically, for $R_{IEX}$= 22.5 µm, we find a maximum of $\partial_\rho c(\rho)$ at $\rho \lesssim R_{IEX}$ of about $\partial_\rho c(\rho) \approx (-3\text{x}10^{-4} / \mu\text{m}^4)[k_0 / \pi D]$ (used in the next section) and *a sublinear decay beyond the maximum* as observed in experiments [1].

## 1.6 Parameter estimates

We now combine the results (16,23) of the previous sections to calculate the saturation value of the slip velocity, both over the glass substrate and the colloidal surface. As a result, we find a saturation value for the solvent advection speed of $v_a$~3.7 µm/s towards the resin and a phoretic speed of the colloids away from the solvent $v_c$~1.1 µm/s. These analytical predictions broadly agree with typical experimental observations [1].

Specifically, from Eq. (23) and $c_{K^+} \approx c^0_{K^+}$ ≈ 1 µmol/L [1] we obtain a saturation value of $\partial_\rho c_{H^+} / c_{K^+} \approx -0.0062\mu\text{m}$ for $k_0$~3.6x10$^8$/s and $D_{H^+} \approx 9.3\mu\text{m}^2/\text{s}$. Using $\varepsilon=\varepsilon_0\varepsilon_r$ with $\varepsilon_r$ = 78.4, $\eta$= 9x10$^{-9}$ kg/(ms) for the fluid viscosity, $T$= 298$K$ and $D_{Cl^-} \approx D_{K^+} \approx 2$ x10$^{-9}$ m$^2$/s and $D_{H^+} \approx 9.3$x10$^{-9}$ m$^2$/s (i.e. $D$ ≈1.67) [1, 4] in Eq. (16) we obtain $\varepsilon kT \text{D}\, \zeta/(4\pi\eta e)$≈ 282 µm$^2$/s for the substrate (zeta potential $\zeta$≈ −100 $mV$) and 113 µm$^2$/s for the colloid ($\zeta$≈ −40 $mV$) and thus an electrophoretic component of fluid advection speed of $v_a^e$ ≈ -1.7 µm/s pointing radially towards the resin along the lower glass plate which is comparable to previous experimental observations; for the slip velocity over the colloidal surface, we find $v_c^e$ ≈ -0.7 µm/s. The 'chemiphoretic' coefficient $\frac{\varepsilon k^2 T^2}{2\pi\eta e^2}\ln(1-\gamma^2)$ amounts to about 67 µm$^2$/s, 12 µm$^2$/s for the substrate and the colloid respectively. Using $c^0_{Cl^-} \approx c^0_{K^+}$, we obtain

$$\partial_r c_{Cl^-} / c_{Cl^-} \approx -(D_{H^+} / D_{Cl^-})\partial_r c_{H^+} / c^0_{K^+} \approx -4.7 c_{H^+} / c^0_{K^+}.$$

This leads to a chemiphoretic component to the slip velocities of −2.0 µm/s and −0.4 µm/s showing that the electrophoretic and the chemiphoretic part of diffusiophoresis in the electrically neutral ionic concentration gradients contribute similarly strongly to the solvent advection speed.

## 1.7 Experimental Details

The ion exchange resin used in this work is micro-gel based cationic ion-exchange resin sphere of diameters 45±1 µm measured by density matching (Purolite Ltd, UK). The model passive particles are commercial, negatively charged, monodisperse polystyrene spheres (PS/Q-F-L1488, MicroParticles GmbH, Germany) stabilized by sulfate surface groups and of diameter 15.2 µm as determined by the manufacturer using electron microscope. Before use, the colloidal particle suspension was diluted and deionized by mixed ion exchange resin (Amberlite K306, Roth GmbH, Germany). Electrophoretic mobility of polystyrene particles was measured by micro-electrophoresis in a home-build Perspex cell (10 mm×10 mm) based on the construction originally

introduced by Uzgiris et al. [5] (see [4] for details). The measured mobility of polystyrene particles is (2.5 ± 0.2) x $10^{-8}$ $m^2/(Vs)$ [4]. The cell for modular swimming was constructed from circular Perspex rings with diameter of $D$= 20 mm attached to a microscopy slide by hydrolytically inert epoxy glue (UHU plus sofortfest, UHU GmbH, Germany) and dried for 24 h before use. Standard ring height was $H$ = 1 mm. Commercial soda lime glass slides of hydrolytic class 3 (VWR International, Germany) served as substrates. They were washed with 1% alkaline solution (Hellmanex ® III, Hellma Analytics) under sonication for 30 min, then rinsed with tap water and subsequently washed with doubly distilled water for several times. The zeta potential of the washed glass slides in deionized water is (105 ± 5) mV [1]. To confine the motion of modular swimmers, arc-shaped periodic microgrooves of a few width (100 µm, 90 µm and 45 µm) and depth 5 µm were patterned on PMMA slides of zeta potential -30 mV [6] by UV lithography. Different sized resins were tried on these microgrooves, and workable size range of groove width to resin diameter is 1.5-10. For direction control by external gravitational field, the $x-y$ position of the sample cell is fixed by a home-made glass chamber. The tilt angle Θ is controlled by spacers of designed heights. For constructing modular swimmers from the resin and passive colloids, a few resins were placed inside the cell followed by injection of 400 µL of deionized colloidal suspension. Then the cell was quickly covered with another glass slide. Colloidal particles quickly settle to the bottom of the cell, where they form a dilute sedimentation layer. Samples were observed by an inverted scientific microscope (DMIRB, Leica, Germany) equipped with a standard video camera. Videos were recorded at a frame rate of 1 Hz and analyzed using a home-written Python script. The velocity of swimmers with different numbers of assembled passive particles and at different tilt angles was averaged over 60-90 complexes.

## 2. References


[1] R. Niu, P. Kreissl, A. T. Brown, G. Rempfer, D. Botin, C. Holm, T. Palberg, J. de Graaf, Soft Matter **13**, 1505 (2017).

[2] D. Prieve, J. Anderson, J. Ebel, M. Lowell, J. Fluid Mech. **148**, 247 (1984).

[3] B. Liebchen, H. Löwen, ArXiv preprint, arXiv:1802.07933 (2018).

[4] R. Niu, D. Botin, J. Weber, A. Reinmüller, T. Palberg, Langmuir **33**, 3450 (2017).

[5] E. Uzgiris and D. Cluxton, Rev. Sci. Instrum. **51**, 44 (1980).

[6] H. Falahati, H. Falahati, L. Wong, L. Davarpanah, A. Garg, P. Schmitz, D. P. J. Barz, Electrophoresis **35**, 870 (2014).
